# Supplementary material for: Anchor-based Robust Finetuning of Vision-Language Models
Source: arXiv:2404.06244 source file (2024-04-09)
Supplement: Supplementary file 1 [file supp_experiments.tex]

\section{Additional Experiments}

Additional experiments are conducted to assess the efficacy of our Anchor-based Robust Finetuning (ARF) in regularizing the finetune process using auxiliary image-text-pair anchors with rich semantics.
Specifically, we provide quantitative results of baselines and our ARF with weight ensemble in Section \ref{sup:ensemble}.
Furthermore, we explore different ways of retrieval in Section \ref{sup:retrieval} and different utilization of anchors in Section \ref{sup:anchors} for domain shift and zero-shot learning scenarios.
Our results demonstrate that the introduced anchors consistently exert a positive influence.
Additionally, our ARF, employing a simple approach, attains exceptional performance in downstream tasks without compromising OOD generalization.

%%%%%%%%%%%%%%%%%%%%%%%%%%%%%%%%%%%%%%%%%%%%%%%%%%%%%%%%%%%%
\begin{table}[ht]
\centering
\resizebox{0.99\linewidth}{!}{
\begin{tabular}{@{}cccccccc@{}}
\toprule
& \multicolumn{7}{c}{ImageNet}\\
\cmidrule{2-8}
% \rotbox{Methods} & \rotbox{ImageNet} & \rotbox{ImageNet-V2} & \rotbox{ImageNet-R} & \rotbox{ImageNet-A} & \rotbox{ImageNet-Sketch} & \rotbox{ObjectNet} & \multicolumn{1}{c}{\rotbox{Avg. Acc}} \\
Methods & \multicolumn{1}{c|}{ID} & Im-V2 & Im-R & Im-A & Im-Sketch & \multicolumn{1}{c|}{ObjectNet} & \multicolumn{1}{c}{Avg. OOD} \\
\midrule
CLIP & \multicolumn{1}{c|}{68.3} & 61.9 & 77.7 & 50.0 & 48.3 & \multicolumn{1}{c|}{54.2} & \multicolumn{1}{c}{58.4} \\
\midrule
LP & \multicolumn{1}{c|}{80.0} & 70.3 & 72.4 & 47.8 & 48.1 & \multicolumn{1}{c|}{53.4} & \multicolumn{1}{c}{58.4} \\
FT & \multicolumn{1}{c|}{82.5} & 72.8 & 74.9 & 48.1 & 51.9 & \multicolumn{1}{c|}{56.5} & \multicolumn{1}{c}{60.8} \\
LP-FT & \multicolumn{1}{c|}{82.1} & 72.8 & 75.3 & 50.1 & 51.7 & \multicolumn{1}{c|}{56.3} & \multicolumn{1}{c}{61.2} \\
FLYP & \multicolumn{1}{c|}{\textbf{82.9}} & \textbf{73.4} & 74.2 & 51.9 & 51.2 & \multicolumn{1}{c|}{56.1} & \multicolumn{1}{c}{61.4} \\
\midrule
ARF & \multicolumn{1}{c|}{82.8} & 73.2 & \textbf{77.2} & \textbf{52.5} & \textbf{53.1} & \multicolumn{1}{c|}{\textbf{57.0}} & \multicolumn{1}{c}{\textbf{62.6}} \\
\bottomrule
\end{tabular}
}
\caption{Domain shift results (\%) of state-of-the-art conventional finetuning and robust finetuning approaches with weight ensemble. We employ ImageNet as the finetuning datasets, while the others serve as domain shift evaluation datasets. The numbers represent the top-1 accuracy and the best results are marked in \textbf{Black}.}
\label{tab:domain}
\end{table}
%%%%%%%%%%%%%%%%%%%%%%%%%%%%%%%%%%%%%%%%%%%%%%%%%%%%%%%%%%%%

\subsection{Quantitative Results of Weight Ensemble}
\label{sup:ensemble}
We compare the performance of our ARF to several baselines in a weight ensembling scenario on domain shift benchmarks.
Ten coefficients, ranging from 0 to 1, are utilized to interpolate the model weights and we select the mixing coefficient with the highest ID validation accuracy.
As illustrated in Table \ref{tab:domain}, our ARF, combined with weight ensembling, achieves the highest domain shift accuracy of 62.6\%, surpassing the previous state-of-the-art method (\textit{i.e.}, FLYP \cite{FLYP}) by 1.2\%.
These findings demonstrate the effectiveness of our ARF when integrated with weight ensemble following Wise-FT \cite{Wise-FT}.

%%%%%%%%%%%%%%%%%%%%%%%%%%%%%%%%%%%%%%%%%%%%%%%%%%%%%%%%%%%%
\begin{table}[ht]
\begin{center}
\resizebox{0.75\linewidth}{!}{
\begin{tabular}{c|cc|c}
\toprule
\multirow{2}{*}{Method}&\multicolumn{2}{c|}{ImageNet}&\multicolumn{1}{c}{Zero-Shot}\\
&ID&Domain Shift&Avg. Acc\\
\midrule
 $ARF_{v \rightarrow v}$ &82.4 &61.0 & 57.1 \\
 $ARF_{t \rightarrow t}$ &82.6 &61.2 & 55.6 \\
 $ARF_{t \rightarrow v}$ &82.5 &61.2 & 55.7 \\
 $ARF_{v \rightarrow t}$ &82.7 &61.3 & 55.6 \\
\bottomrule
\end{tabular}
}
\end{center}
\vspace{-2mm}
\caption{Ablation study for different ways of retrieval in our ARF. We use the first letter in the subscript to denote the modality in the finetune set, and the second letter in the subscript to represent the modality in the candidate set. For instance, the image-to-text retrieval of our ARF is denoted as $ARF_{v \rightarrow t}$.}
\label{tab:retrieval}
\end{table}
%%%%%%%%%%%%%%%%%%%%%%%%%%%%%%%%%%%%%%%%%%%%%%%%%%%%%%%%%%%%

\vspace{-2mm}
\subsection{Different Ways of Retrieval}
\label{sup:retrieval}
In addition to cross-modal retrieval capacity, CLIP can also search for image-text pairs relevant to the downstream task from the candidate set using uni-modal retrieval.
Specifically, as depicted in Fig.\ref{fig:retrieval}, four different combinations of retrieval between images and texts from the downstream dataset and the candidate set are investigated to identify appropriate content for preserving the OOD generalization capabilities of CLIP.
We denote the image-to-text retrieval as $ARF_{v \rightarrow t}$, which utilizes images from the finetune set to search for the most similar texts in the candidate set.

As presented in Table \ref{tab:retrieval}, it can be observed that $ARF_{v \rightarrow v}$ achieves the highest accuracy in zero-shot learning but exhibits the lowest performance in ID and domain shift scenarios.
This is because uni-modal retrieval, using merely visual information, may search for image-text pairs unrelated to the downstream task while possessing more diverse semantics, thereby improving zero-shot prediction at the expense of ID and domain shift accuracies.
Regarding the other three retrieval combinations, they identify appropriate image-text pairs and yield similar results, demonstrating the exceptional retrieval capacity of CLIP.
For the highest ID performance, we choose $ARF_{v \rightarrow t}$ as our approach.

\subsection{Different Utilization of Anchors}
\label{sup:anchors}
\noindent\textbf{Different Utilization of Text-Compensated Anchors.}
%we employ a contrastive loss function $\mathcal{L}_{\text{Cap}}$ to separately align text-compensated anchors (\textit{i.e.}, captions) and images from the finetune set.
In our ARF, the captions generated by the Text-Compensated Anchor Generation module and class prompts are aligned separately with the images from the finetune set.
This strategy effectively avoids overfitting by preventing the image from being drawn excessively close to its corresponding class prompt.
We designate this approach as $sep(t_c, t^{\text{cap}})$, where $t_c$ denotes the class prompts and $t^{\text{cap}}$ represents the generated captions.
Alternatively, we can also merge the class prompt with the caption to enhance the text representation, such as ``a photo of a \texttt{[CLASS]}, \texttt{[CAPTION]}'', where ``\texttt{[CLASS]}'' indicates the class name and ``\texttt{[CAPTION]}'' refers to the text description generated by a pretrained captioner for each image. 
This approach of employing the text-compensated anchor is denoted as $merge(t_c, t^{\text{cap}})$.

%%%%%%%%%%%%%%%%%%%%%%%%%%%%%%%%%%%%%%%%%%%%%%%%%%%%%%%%%%%%
\begin{table}[t]
\begin{center}
\resizebox{0.85\linewidth}{!}{
\begin{tabular}{c|cc|c}
\toprule
\multirow{2}{*}{Method}&\multicolumn{2}{c|}{ImageNet}&\multicolumn{1}{c}{Zero-Shot}\\
&ID&Domain Shift&Avg. Acc\\
\midrule
\multicolumn{1}{c|}{baseline}&82.6 &59.4 & 48.6 \\
\midrule
 $merge(t_c, t^{\text{cap}})$ &82.6 &60.5 & 53.4 \\
 $sep(t_c, t^{\text{cap}})$ &82.6 &60.7 & 54.3 \\
\midrule
 $merge(t^{\text{cap}}, t^{\text{ret}})$ &82.7 &61.3 & 54.3 \\
 $sep(t^{\text{cap}}, t^{\text{ret}})$ &82.7 &61.3 & 55.6 \\
\bottomrule
\end{tabular}
}
\end{center}
\caption{Ablation study for different utilization of anchors in our ARF. The baseline only conducts visual-language contrastive learning for finetuning like FLYP \cite{FLYP}.}
\label{tab:anchor}
\end{table}
%%%%%%%%%%%%%%%%%%%%%%%%%%%%%%%%%%%%%%%%%%%%%%%%%%%%%%%%%%%%

As demonstrated in Table \ref{tab:anchor}, we can see that both approaches significantly improve the performance of zero-shot learning and domain shift over the baseline, indicating the effectiveness of our strategy in mitigating overfitting through the use of text-compensated anchors. 
The separate alignment of captions and class prompts with images denoted as $sep(t_c, t^{\text{cap}})$, achieves better performance compared to $merge(t_c, t^{\text{cap}})$, with improvements of 0.9\% and 0.2\% in zero-shot learning and domain shift, respectively. 
Therefore, we employ $sep(t_c, t^{\text{cap}})$, this straightforward utilization of text-compensated anchors, in our ARF.

\noindent\textbf{Different Utilization of Retrieved Image-Text Anchors.}
% Regarding the utilization of retrieved image-text-pair anchors, we apply contrastive loss $\mathcal{L}_{\text{Ret}}$ to regularize the finetune process and we denote this approach as $sep(t_c, t^{\text{ret}})$.
% % Here, $\textit{ret}$ represents the retrieved image-text pairs.
% Alternatively, we can merge the retrieved image-text anchors with the text-compensated anchors in a mini-batch to finetune the CLIP model, referring to this strategy as $merge(t_c, t^{\text{ret}})$.
We apply two separate contrastive losses (\textit{i.e.}, $\mathcal{L}_{\text{Cap}}$ and $\mathcal{L}_{\text{Ret}}$) to align the text-compensated anchors and the retrieved image-text anchors, denoting this approach as $sep(t^{\text{cap}}, t^{\text{ret}})$. Alternatively, we can merge the two types of anchors in a mini-batch and calculate a single contrastive loss for finetuning the CLIP model, referring to this strategy as $merge(t^{\text{cap}}, t^{\text{ret}})$.

As shown in Table \ref{tab:anchor}, it is evident that $sep(t^{\text{cap}}, t^{\text{ret}})$ significantly improves the performance of zero-shot learning and domain shift compared to the addition of text-compensated anchors.
In contrast, $merge(t^{\text{cap}}, t^{\text{ret}})$ merely boosts performance on domain shift.
This finding suggests that aligning the retrieved image-text pairs separately using contrastive loss more effectively maintains the original feature space of CLIP while merging the retrieved image-text pairs with the image-caption pairs in a mini-batch mitigates its effectiveness. 
Consequently, we employ $sep(t^{\text{cap}}, t^{\text{ret}})$ in our ARF.
